# Supplementary material for: Joint Scoring Rules: Zero-Sum Competition Avoids Performative Prediction
Source: arXiv:2412.20732 ancillary file (2024-12-30)
Supplement: Supplementary file 1 [file Technical_Appendix.pdf]

# Joint Scoring Rules: Zero-Sum Competition Avoids Performative Prediction Technical Appendix

Rubi Hudson*

## Appendix A: Proofs

### Main Results

**Lemma 1.** *Under a zero-sum scoring rule $S$, all agents receive an expected score of* 0 *in any equilibrium.*

In the main paper, we assume $c = 0$.

*Proof.* Proof: For each action, an agent's expected score is:

$$s(p_{i,a}, q_a) - \frac{\sum_{j \neq i} s(p_{j,a}, q_a)}{n-1} + c$$

Since $s$ is a strictly proper scoring rule, $s(\cdot, q_a)$ is maximized by $p_{i,a} = q_a$ and so $s(q_a, q_a) - \frac{\sum_{j \neq i} S'(p_{j,a}, q_a)}{n-1} \geq c$.
This means that in any equilibrium each agent's expected score is at least $c$. Since scores are zero-sum, it must be that each agent's expected score is exactly $c$. □

**Theorem 2.** *When $n \geq 2$, the combination of the optimistic-max decision rule $D$ and a zero-sum scoring rule $S$ is quasi-strictly proper, and in any equilibrium the max decision rule applied to any agent selects action $a^*$.*

*University of Toronto

*Proof.* First, we show that in equilibrium, $\nexists p_{i,a}$ such that $p_{i,a} \succ q_{a^*}$. Suppose $p$ is an equilibrium, and such a prediction exists. Based on the decision rule, the principal must end up choosing some action $a'$ where $\exists p_{j,a'} \succ q_{a^*}$. Then, since the decision rule is optimistic, there exists some agent $k \neq j$ who is either reporting honestly or can change their prediction to $p_{k,a'} = q_{a'}$ without affecting the action taken. The score for such a prediction, $S_k(a', (q_{a'}, p_{-(k,a')}), q)$, is equal to

$$s(q_{a'}, q_{a'}) - \frac{s(p_{j,a'}, q_{a'})}{n-1} - \frac{\sum_{i \neq j,k} S'(p_{i,a'}, q_{a'})}{n-1} > 0$$

The inequality follows because $s(\dot{;}q_{a'})$ is uniquely maximized at $q_{a'}$, and $p_{j,a'} \neq q_{a'}$. By Lemma 1, this contradicts that $p$ is an equilibrium.
Next, we show that in equilibrium, $\nexists i$ such that $q_{a^*} \succ p_{i,a^*}$. Suppose $p$ is an equilibrium, and such a prediction exists. If another agent $j \neq i$ reports honestly, then $D(p) = a^*$ since the decision rule is optimistic and we have previously established that no predictions are more preferred to $q_{a^*}$. The score for such a prediction, $S_k(a', (q_{a^*}, p_{-(j,a^*)}), q)$, is equal to

$$s(q_{a^*}, q_{a^*}) - \frac{s(p_{i,a'}, q_{a^*})}{n-1} - \frac{\sum_{k \neq i,j} S'(p_{k,a^*}, q_{a^*})}{n-1} > 0$$

By Lemma 1, this contradicts that $p$ is an equilibrium.
In equilibrium, each agent reports honestly for $a^*$ and there are no reports $p_{i,a} \succ q_{a^*}$, so running the max decision rule on any $p_i$ must choose $a^*$. Using the optimistic-max decision rule across agents similarly chooses $a^*$. Predictions conditional on untaken actions do not enter the scoring function, and so honesty is weakly incentivized. As such, the decision/scoring rule pair is quasi-strictly proper. □

**Theorem 3.** *When $n = 2$, for a principal with preferences that follow Independence, the combination of the mean-max decision rule and a zero-sum scoring rule is quasi-strictly proper*

*Proof.* We refer to the mean-max decision rule as $D$ and the linearly zero-sum scoring rule as $S$, with $c = 0$ chosen for simplicity.
By Lemma 1, both agents receive an expected score of zero in any equilibrium.
First, we show that in equilibrium, $\nexists i, a$ such that $p_{i,a} \succ q_{a^*}$. Suppose such a prediction exists. Let $\bar{a}_i$ be a most preferred action according to the predictions of agent $i$, such that $p_{i,\bar{a}} \succsim p_{i,a}$, $\forall a$. If agent $j \neq i$ predicts

$p_{j,a} = q_{\bar{a}}$, $\forall a$, then by Independence action $\bar{a}$ will be chosen and agent $j$ will receive a positive score, contradicting that this is an equilibrium. Next, we show that in equilibrium, $\nexists i$ such that $q_{a^*} \succ p_{i,a^*}$. Suppose such a prediction exists. If agent $j \neq i$ predicts $p_{j,a} = p_{i,a^*}$, $\forall a \neq a^*$, and $p_{j,a^*} = q_{a^*}$, then by Independence $a^*$ will be chosen and agent $j$ will receive a positive score, contradicting that this is an equilibrium.
In equilibrium, each agent reports honestly for $a^*$ and there are no reports $p_{i,a} \succ q_{a^*}$, so running the max decision rule on any $p_i$ must choose $a^*$. Using the mean-max decision rule across agents similarly chooses $a^*$. Predictions conditional on untaken actions do not enter the scoring function, and so honesty is weakly incentivized. As such, the decision/scoring rule pair is quasi-strictly proper. □

**Theorem 4.** *When $n \geq 2$, for a principal with preferences that follow Independence, the combination of the mean-max decision rule and a zero-sum scoring rule is quasi-strictly proper when restricting to strong equilibria.*

*Proof.* Identical to the proof of Theorem 3 , replacing lone agent $j$ with a coalition of size $n - 1$. □

**Theorem 5.** *If $n \geq 2$, the combination of a disagreement-seeking-max decision rule and a zero-sum scoring rule is strictly proper, and the principal deterministically chooses $a^*$.*

*Proof.* We refer to the disagreement-seeking-max decision rule as $D$ and the linearly zero-sum scoring rule as $S$, with $c = 0$ chosen for simplicity.
By Lemma 1, all agents receive an expected score of zero in equilibrium. As such, there can be no equilibrium where there exists some $p_{i,a} \neq q_a$. Suppose there was. Then, another agent reporting $p_j = q$ is then guaranteed a positive expected score, as an action where agents disagree will be chosen, contradicting that this is an equilibrium.
Since all agents report honestly for all actions, the scoring rule is strictly proper. Then, the principal is always able to select $a^*$. □

**Theorem 6.** *If a symmetric scoring rule/decision rule pair is quasi-strictly proper, then the scoring rule is zero-sum.*

*Proof.* For a quasi-strictly proper scoring rule/decision rule pair, $p = \mathbf{q}$ must be an equilibrium, as all agents report honestly for $a^*$, $a^*$ is chosen, and all agents are weakly incentivized for honesty in all predictions. This means

that if $p_i = \tilde{p}$, $\forall i$, then the principal must decide using the max decision rule. If not, then there would exist some $q$ for which they do not select $a^*$.

This means that the scores must be the same in each equilibrium. If they are not, then for some set of preferences either there exists an equilibrium where $a^*$ is not chosen or $\mathbf{q}$ is not an equilibrium, which both contradict being quasi-strictly proper. By symmetry, all agents receive the same score for any action.

As $a^*$ can be any distribution for some set of preferences, and each agent reports it honestly, they must face a proper scoring rule when conditioning on the action chosen and the predictions from other agents. So, for a given action, the other predictions must induce a strictly monotonic transformation of a proper scoring rule. By symmetry, the same monotonic transformation is applied to all of them, which means that for any base score, the transformation must map it to the same constant. The only transformation which does this is the form $S_i(a, p, q) = s(p_{i,a}, q_a) - \frac{\sum_{j \neq i} s(p_{j,a}, q_a)}{n-1} + c$. As such, the scoring rule must be zero-sum □

## Efficient Search Proofs

**Theorem 7.** *A principal can identify $a^*$ with at most $O(log(|\mathcal{A}|))$ comparisons between actions.*

*Proof.* Set the constant term of the zero scoring rule to $c = 0$.

The principal proceeds as follows: they start by splitting the set of actions into two subsets of equal size (or with a one element difference). They then elicit conditional predictions for the actions of continuing the procedure with each subset. Based on these predictions, the principal selects a set to take an action from and discards the other. If the chosen set only has one action in it, they take that action, otherwise they repeat the procedure on that set. It is clear that this takes $O(log(|\mathcal{A}|))$ comparisons. It remains to show that this procedure selects $a^*$. We will show this via induction on the size of the two sets that are compared.

As the base case, if both sets have size 1, then by Theorem 2, the decision maker will choose the more preferred action.

For the inductive hypothesis, assume that the procedure works for comparing sets of actions up to size $m - 1$. Consider two sets of actions, $A_1$ and $A_2$, that each have up to $m$ elements. Running the procedure on $A_1$ will involve splitting them up into sets of size less than or equal to $m - 1$, which by the

inductive hypothesis results in the best action from $A_1$, denoted $a_1^*$ being chosen. The equivalent holds if the procedure is run on $A_2$. So, choosing between $A_1$ and $A_2$ is equivalent to choosing between $\{a_1^*\}$ and $\{a_2^*\}$, which by Theorem 2 chooses the more preferred, which is the most preferred in $A_1 \cup A_2$. □

**Theorem 8.** *A principal can identify $a^*$ with at most $O(1)$ comparisons between actions.*

*Proof.* Set the constant term of the zero scoring rule to $c = 0$.
Consider the following procedure. An agent, indexed to 1, is randomly assigned to choose an action, $\tilde{a} \in \mathcal{A}$. The principal then creates two sets, $A_1 = \{\tilde{a}\}$ and $A_2 = \mathcal{A} \backslash \tilde{a}$ and runs the procedure from the proof of Theorem 7 (also outlined in Algorithm 1 of the main paper). If $\tilde{a}$ is selected, the agent who chose it receives an additional constant payoff of $k > 0$.
Agent 1's payoff is maximized at $k$ by choosing $a^*$, as it is the only one for which they can report honestly and still have it be chosen. Choosing a different option and reporting dishonestly so that it is chosen earns $k$ but with a strictly negative score for some predictions, while choosing a different option and reporting honestly so that it is not selected earns a score of 0.
If $\tilde{a} = a^*$, they select it after a single comparison and the procedure ends. As such, it takes $O(1)$ steps. □

## Stochastic Choice Proofs

For reference, the condition used in the proofs for this section are as follows:

**Condition 1.** *If $p'_{i,a} \succ p_{i,a}$ $\forall a \in A \subseteq \mathcal{A}$ and $p_{-(i,A)} = p'_{-(i,A)}$, then $\exists a \in A$ such that $D_a(p) > 0$, implies $\exists a' \in A$ such that $D_{a'}(p') > 0$*

**Condition 2.** *If $p_{-(i,a)} = p'_{-(i,a)}$, $p_{i,a} \succ p'_{i,a}$ then for $a' \neq a$ $D_{a'}(p) > 0$ implies $D_{a'}(p') > 0$*

**Condition 3.** *If $p_{-(i,a)} = p'_{-(i,a)}$ and $D_a(p) = D_a(p') = 0$ then $D(p) = D(p')$*

**Lemma 9.** *Under a zero-sum scoring rule $S$ and optimistic decision rule $D$, if Conditions 1 and 2 are met then in equilibrium $p$ $\forall i, \forall a$ such that $D_a(p) > 0$, $p_{i,a} = q_a$*

*Proof.* Lemma 1 shows that in any equilibrium, $E_{a \sim D(p)}[S_i(a, p, q)] = c$, $\forall i$. First we show that in equilibrium, $\forall a$ such that $D_a(p) > 0$, $S_i(a, p, q) = c$ $\forall i$. Suppose this were not the case for some $i, a$. Then there exists some agent $j$ such that $S_j(a, p, q) < c$. Since $E_{a \sim D(p)}[S_i(a, p, q)] = c$, $\exists a'$ such that $S_j(a', p, q) > c$ and $D_{a'}(p) > 0$.
Consider agent $j$ changing their prediction to $p'_{j,a} = q_a$, $\forall a \in \underline{A} \equiv \{a | S_j(a, p, q) < c\}$. Start by making the update for all $a \in \underline{A}$ where $q_a \succ p_{j,a}$ and $\exists i$ such that $p_{i,a} = q_a$. By the optimistic decision rule, the probabilities assigned to all actions remain the same. Next, make the update for all $a \in \underline{A}$ where $q_a \succ p_{j,a}$ and $\nexists i$ such that $p_{i,a} = q_a$. By Condition 1, at least one action with expected score strictly greater than $c$ is assigned positive probability. Finally, make the update for all $a \in \underline{A}$ where $p_{j,a} \succ q_a$. By Condition 2, all other actions assigned positive probability continue to be assigned positive probability.
Since all predictions for actions with an expected score less than $c$ were changed to the optimal prediction for that action, each action has an expected score of at least $c$. At least one action assigned positive probability has an expected score strictly greater than $c$, so the overall expected score is strictly greater than $c$, contradicting that this is an equilibrium by Lemma 1. Therefore, $\forall a$ such that $D_a(p) > 0$, $S_i(a, p, q) = c$ $\forall i$.
Finally, we show that in equilibrium, this means $\forall a$ such that $D_a(p) > 0$, $p_{i,a} = q_a$, $\forall i$. Suppose not. If there exists $i$ such that $p_{i,a} \succ q_a$, then any other agent $j$ can predict $p_{j,a} = q_a$, which does not change the decision probabilities due to the optimistic decision rule, and receive a positive expected score. If $q_a \succ p_{i,a}$, $\forall i$, then any agent $j$ can predict $p_{j,a} = q_a$, which by Condition 1 does not change the probability of action $a$ to zero, and receive a positive expected score. Either way, the equilibrium is contradicted. So, $\forall a$ such that $D_a(p) > 0$, $p_{i,a} = q_a$, $\forall i$. □

**Theorem 10.** *When $n \geq 2$, a zero-sum scoring rule and the random-max decision rule is quasi-strictly proper.*

*Proof.* Since the principal will only take an action that is reported as best by at least one agent, this decision rule trivially meets Conditions 1 and 2, so by Lemma 9, in equilibrium all agents report honestly for all actions taken with positive probability. If at least one agent reports honestly for $a^*$, it will be taken with positive probability meaning that all agents will report honestly for $a^*$. If no agents report honestly for $a^*$, then an agent reporting honestly for all actions would result in $a^*$ being taken with positive probability and

so would receive an expected score higher than $c$, which contradicts that it is an equilibrium as per Lemma 1.
No agent reports $p_{i,a} \succ q_{a^*}$, as this would result in some action for which they are misreporting being taken with positive probability, contradicting Lemma 9. As $a^*$ is thus taken deterministically in all equilibria, agents predict honestly for it, and there is no incentive for dishonesty on untaken actions, this scoring/decision rule pair is quasi-strictly proper. □

**Theorem 11.** *When $n \geq 2$, for a principal with preferences that follow Independence, a zero-sum scoring rule and the random-mean-max decision rule is quasi-strictly proper.*

*Proof.* Conditions 1 and 2 are met, since by Independence an agent increasing how much the principal prefers the prediction for some action in the principal choosing that action or no change. Therefore, Lemma 9 applies, and in equilibrium all agents report honestly for all actions taken with positive probability.
If at least one agent reports honestly for $a^*$, it will be taken with probability at least $\epsilon^{n-1}$ meaning that all agents will report honestly for $a^*$. If no agents report honestly for $a^*$, then an agent reporting honestly for all actions would result in $a^*$ being taken with positive probability and so would receive an expected score higher than $c$, which contradicts that it is an equilibrium as per Lemma 1.
No agent reports $p_{i,a} \succ q_{a^*}$, as this would result in some action for which they are misreporting being taken with positive probability, contradicting Lemma 9. As $a^*$ is thus taken deterministically in all equilibria, agents predict honestly for it, and there is no incentive for dishonesty on untaken actions, this scoring/decision rule pair is quasi-strictly proper.

□

**Theorem 12.** *Under a zero-sum scoring rule $S$ and optimistic decision rule $D$ meeting Conditions 1-3, then in any equilibrium $p$, $D(p) = D(\boldsymbol{q})$*

*Proof.* Let $A_+ \equiv \{a \in A | D_a(q, ..., q) > 0\}$ and $A_0 \equiv \{a \in A | D_a(q, ..., q) = 0\}$. We will show that in any equilibrium, $D_a(p) > 0$ if and only if $a \in A_+$.
First we show that in equilibrium, $D_a(p) = 0$, $\forall a \in A_0$. Suppose not, for some non-empty set of actions $A' \subseteq A_0$. Lemma 9 means that $p_{i,a} = q_a$, $\forall a \in A'$. Condition 3 says that no $p_{i,a'}$ for $a' \in A_0 \backslash A'$ affects $D_a(p)$, so some $a'' \in A_+$ must be misrepresented. Again by Lemma 9, there can

be no misrepresentations for actions assigned positive probability, so the misrepresented action(s) must have $D_{a''}(p) = 0$. Call the set of these actions for $A'' \subseteq A_+$. The optimistic decision rule means that all agents must be misrepresenting all $a'' \in A''$. If one agent $i$ switched to reporting $p'_{i,a''} = q_{a''}$ $\forall a'' \in A''$ then by the optimistic decision rule all $a \in A_+ \cup A'$ are treated as though they received an accurate prediction. Since by Condition 3 no $a' \in A_0 \backslash A'$ affects $D_a(p)$, we must have that $D(p') = D(q, ..., q)$ and their expected score for the agent who switched would be positive, so this cannot be an equilibrium.

Next, we show that in equilibrium $D_a(p) > 0$, $\forall a \in A_+$. Suppose not, for some non-empty set of actions $A'' \subseteq A_+$. Since $D_{a'}(p) = 0$, $\forall a' \in A_0$, Lemma 9 and Condition 3 mean that this must be due to misrepresentation of actions in $A''$. These misrepresentations cannot all make the actions appear better than they are, as in that case Condition 1 would mean at least one was assigned positive probability, which is ruled out by 9. However, if at least one action is made to appear worse than it is, then by the optimistic decision rule all agents are reporting it as worse, and so any agent reporting $p'_{i,a''} = q_{a''}$ $\forall a'' \in A''$ would ensure that at least one misreported action is assigned positive probability, thus giving them positive expected score and showing that this cannot be an equilibrium either.

All actions in $A_+$ are assigned positive probability, and all actions in $A_0$ are assigned zero probability. Lemma 9 means that all reports for actions in $A_+$ are honest, and Condition 3 means that the probabilities reported for actions in $A_0$ do not affect the decision function, so $D(p) = D(q, ..., q)$. □

# Appendix B: Experiments

## Description of Experiments

To generate the ground truth in our toy model, we instantiate a gold standard neural network that takes in eight context variables and eight action variables (restricted to be one-hot vector of length eight), and outputs a distribution over eight outcomes by taking a softmax over the output later.

Our gold standard model has a single hidden layer of 1,024 neurons. There is also a skip connection from the actions to the output layer, multiplied by a constant, so that the actions have a considerable impact on the probabilities and performativity is possible. This constant was tweaked through experi-

mentation to strike the right balance between the context and action both impacting the resulting distribution.

The context variables are randomly generated according to a uniform distribution, and then repeated eight times as they are combined with each of the eight actions. All eight actions for each context always appear adjacent to each other in the same batch, representing conditional predictions being made for all eight actions. We train the models on $2^{16}$ contexts for each experiment, divided into batches of sixty-four.

The trained neural nets have four layers of sixty-four neurons. Dropout is applied to the context part of the input (but not the actions) at a rate of 25%, and to the hidden layers at a rate of 50%. The same mask is applied to all eight inputs that contain a particular context.

The models are trained with the Adam optimizer, minimizing expected cross-entropy loss conditional on the action taken. Each gradient update consists of two forward passes with different masks on each input, to keep all training methods consistent with training under a (non-exact) zero-sum objective where two forward passes are required.

The principal is assigned a random utility function, with the utility assigned to each outcome following a Normal distribution. The utilities are then normalized and multiplied by a constant, so that the preferred action is taken considerably more often but not close to exclusively. They then stochastically choose an action by taking a softmax over the expected utility.

For Experiment 1, the three techniques being compared are applied to the same randomly instantiated neural net.

For Experiment 2, the techniques are applied to a model trained in a performative environment without intervention. To create higher amounts of performativity, we drop the temperature of the decision maker's randomization throughout the training, and the techniques being compared for untraining purposes are used in the lowest temperature environment.

In running each experiment, we repeat the training process sixty-four times, for each combination of sixteen utility functions and four gold standard models. The average statistics for each of the batch are presented.

## Results and Robustness Checks

The results for the main experiments are included in the main paper, but repeated here for completeness.

Experiment 1:

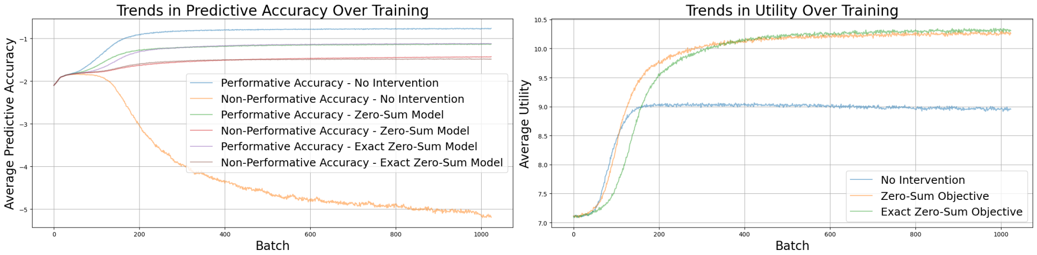


Experiment 2:

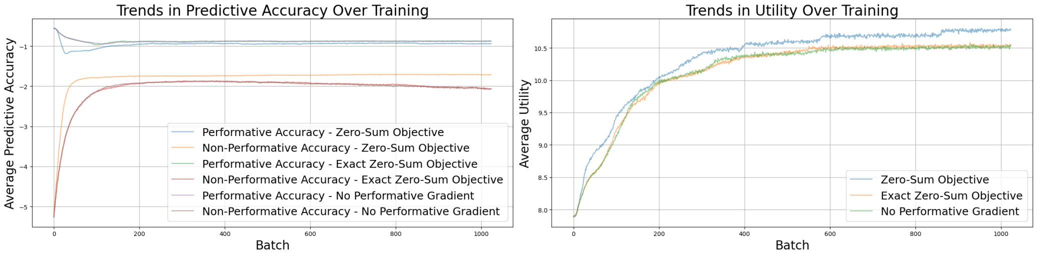


We also track the probability of the principal taking their most preferred action over time.

Experiment 1:

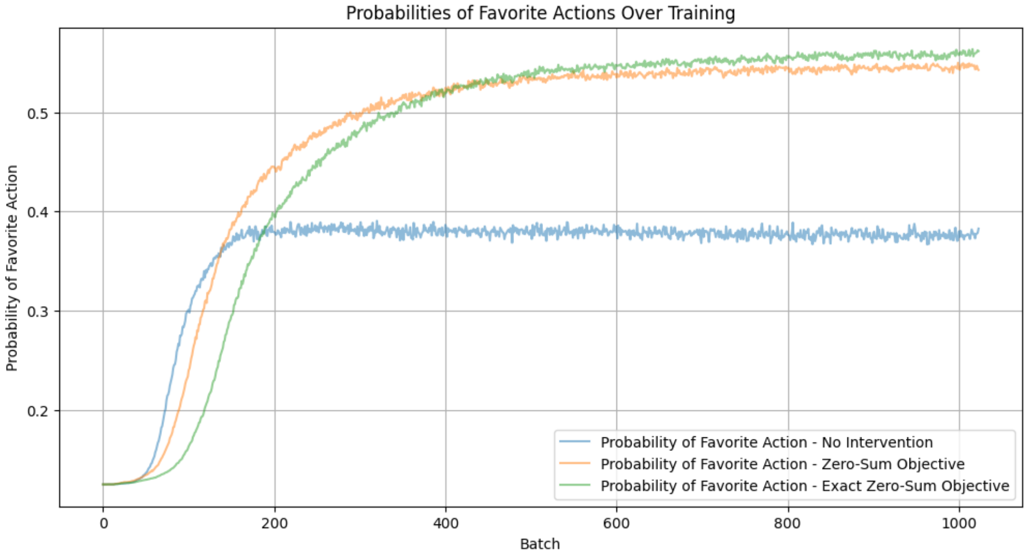

Experiment 2:

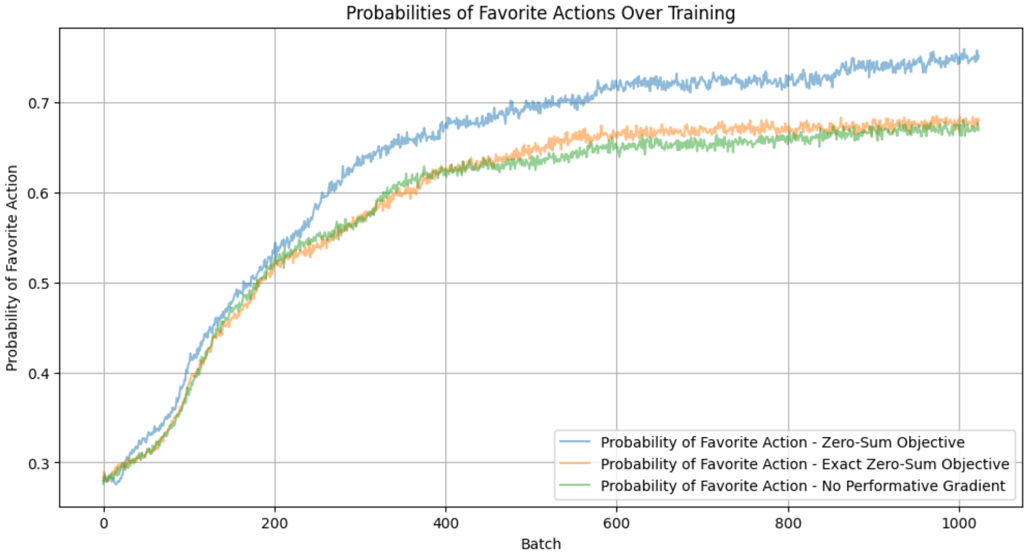


The chance of choosing the most preferred action very closely follows the trend of utility throughout training.

We run robustness checks to ensure that the above results are not due to experimental decisions. We test whether performativity was learned by the variant version of the model trained with a (non-exact) zero sum objective. The variants we test are using a mean decision rule, restricting the decision softmax to the top four options, using the Brier score, using eight agents, and pretraining on historical data.

**Mean Decision Rule:**

We try changing the decision rule used from one that takes the softmax based on the expected utility of the optimistic prediction to one that takes the softmax based on the expected utility from the mean predictions.

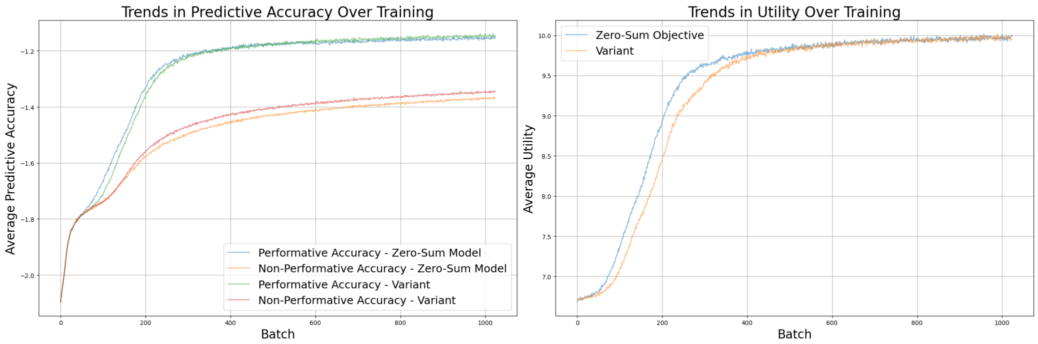


This update results in almost no change. The mean decision rule results in very slightly more accuracy on average, while performative accuracy and the principal's utility rise slightly more slowly under the mean decision rule, but still converge to the same point.

**Top Four:**
We try changing the decision rule so that only the top four of eight actions actions by expected utility are assigned positive probability.

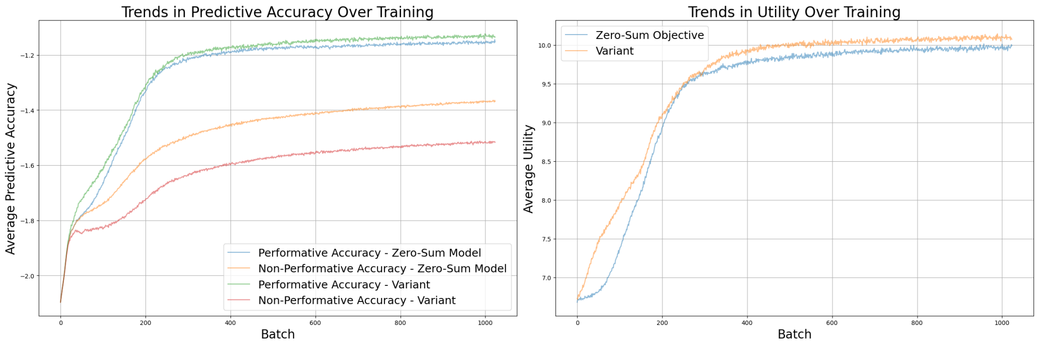


This updates results in less average prediction accuracy, and slightly less performative accuracy but slightly more utility. The decrease in predictive accuracy is intuitive, as the model is no longer trained on low utility actions. The increase in utility can be explained by the reassignment of probability from the bottom four actions by expected utility to the top four.

**Brier Score:**
We try changing the base scoring rule used from the log score to the Brier score.

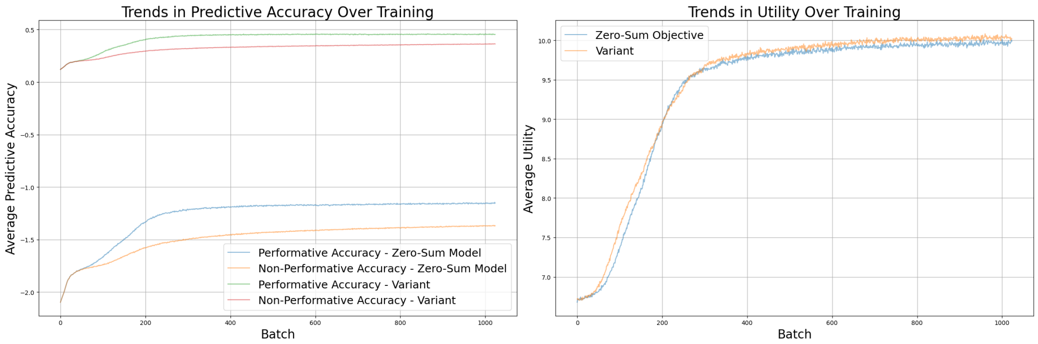


The trends in average predictive accuracy and performative accuracy are roughly the same shape, with the remaining differences coming from the different ranges of scores that each scoring rule assigns.

**Eight Agents:**

We try calculating the zero-sum objective using eight agents, rather than two.

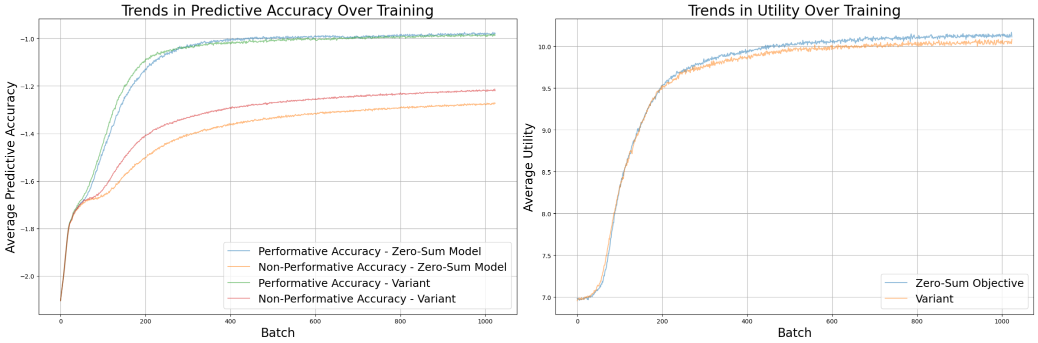


We see that using additional agents results in the same levels of predictive accuracy, but slightly higher levels of average predictive accuracy and utility. Note that in this variant, additional compute was required by the variant training process in order to run the extra agents.

**Pretraining:**

We try pretraining the model using historical data before training it in the environment incentivizing performativity. Here, the comparison to only the original zero-sum objective would not be intuitive, so we instead include all of the training processes starting from the pretrained model. For comparison, see the results of Experiment 1 above.

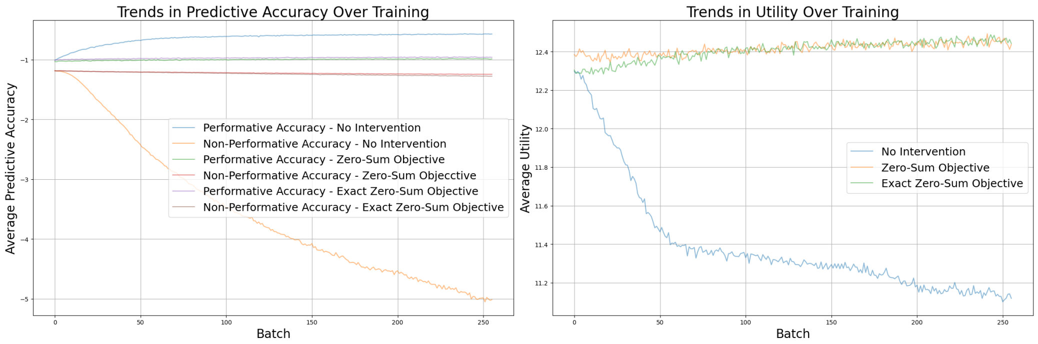


We see that the pretraining imparts most of the predictive accuracy into the model. Once switched into the environment incentivizing performativity, the zero-sum models stay constant in both measures of predictive accuracy, while the model with no intervention increases performative accuracy at the expense of average accuracy.

As we can see through these robustness checks, the choices made in the training of the model can have minor effects, but the main takeaway is that the zero-sum objectives resist becoming performative in all cases.
